# Supplementary material for: Paradigm Shift in Infrastructure Inspection Technology: Leveraging High-performance Imaging and Advanced AI Analytics to Inspect Road Infrastructure
Source: arXiv:2505.13955 source file (2025-05-20)
Supplement: Supplementary file 1 [file 10_appendix.tex]

\appendix

\section{algorithm}

\begin{figure}[t]
\begin{algorithm}[H]
\flushright
\begin{minipage}{0.95\linewidth}
\caption{Offset-scan Back-projection algorithm layout before and after optimization. 
}
\label{alg:BPOpt}
\small
\LinesNumbered
\KwIn{Before optimization $input[N_v][N_r][N_c]$ projections.}
\KwOut{Before optimization $output[N_z][N_y][N_x]$ volume.}

{
% \normalem

\For{$y=0$ \textbf{to} $N_y$}{

    \For{$x=0$ \textbf{to} $N_x$}{

        \For{$z=0$ \textbf{to} $N_z$}{
        
            val = 0.0; \Comment{\textcolor{blue}{//Scalar}}
            
            \For{$v=0$ \textbf{to} $N_v$}{
            
                $\mathrm{i_{det}}$ = Proj(x, y, v);
                
                val += input[v][z][$\mathrm{i_{det}}$]; \Comment{\textcolor{blue}{//Scalar}}
                
            }
            output[z][y][x] = val; \Comment{\textcolor{blue}{//Scalar}}

        }
    }
}
}

\KwIn{After optimization $input[N_c][N_v][N_r]$ projections.}
\KwOut{After optimization $output[N_y][N_x][N_z]$ volume.}

{
% \normalem
    
\For{$yy=0$ \textbf{to} $N_y$ \textbf{step} $N_{y\_block}$}{

    \For{$xx=0$ \textbf{to} $N_x$ \textbf{step} $N_{x\_block}$}{
    
        \For{$y=0$ \textbf{to} $N_{y\_block}$}{
        
            \For{$x=0$ \textbf{to} $N_{x\_block}$}{

                $\mathrm{y_{det}}$ = yy * $N_{y\_block}$ + y; 
                
                $\mathrm{x_{det}}$ = xx * $N_{x\_block}$ + x;
        
        \For{$z=0$ \textbf{to} $N_z$}{

            val[z] = 0.0; \Comment{\textcolor{blue}{//Vector}}
        }
        
        \For{$v=0$ \textbf{to} $N_v$}{

            $\mathrm{i_{det}}$ = Proj($\mathrm{x_{det}}$ $\mathrm{y_{det}}$, v);

            \For{$z=0$ \textbf{to} $N_z$}{
                
                val[z] += input[$\mathrm{i_{det}}$][v][z]; \Comment{\textcolor{blue}{//Vector}}
                
            }
        }
        
        \For{$z=0$ \textbf{to} $N_z$}{
        
            output[$\mathrm{y_{det}}$][$\mathrm{x_{det}}$][z] = val[z]; \Comment{\textcolor{blue}{//Vector}}
            
        }
        }
        }

        }
    }
}
}

\end{minipage}
\end{algorithm}

\end{figure}
